# Supplementary material for: Double Configuration Interaction Singles: Scalable and size-intensive approach for orbital relaxation in excited states and bond-dissociation
Source: arXiv:2410.09912 ancillary file (2024-12-13)
Supplement: Supplementary file 1 [file DCIS_SI.pdf]

# Supporting Information for "Double Configuration Interaction Singles: Scalable and size-intensive approach for orbital relaxation in excited states and bond-dissociation"

Takashi Tsuchimochi*
*College of Engineering, Shibaura Institute of Technology,*
*3-7-5 Toyosu, Koto-ku, Tokyo 135-8548 Japan and*
*Institute for Molecular Science, 38 Nishigonaka, Myodaiji, Okazaki 444-8585 Japan*

* tsuchimochi@gmail.com

## I. Analytical expressions of matrix elements and sigma vectors

We first note that, in the following, we formulate our derivation as general as possible, so that we can easily generalize these results to the spin-unrestricted regime, or even to the non-Hartree-Fock reference. Therefore, the orbital indices stand for spin-orbitals but not spatial-orbitals, and the Fock matrix $\mathbf{F}$ may not be diagonal.

### A. Energy and overlap

The $I$th CIS wave function is given by

$$|0_I\rangle = \sum_\mu c_\mu^I |\Phi_\mu\rangle \tag{S1}$$

where $\mu \in \{0, ai\}$ indicate the Hartree-Fock determinant ($|\Phi_0\rangle$) and singly excited determinants $|\Phi_i^a\rangle$. Note that, if the HF state is stationary, $c_0^I = 0$.

The CIS energy is given by

$$E_{0,I} = \frac{\langle 0_I|\hat{H}|0_I\rangle}{\langle 0_I|0_I\rangle} \tag{S2}$$

The numerator and denominator are

$$H_{IK} := \langle 0_I|\hat{H}|0_K\rangle = E_{\mathrm{HF}} N_{IK} + \mathrm{Tr}\left[\mathbf{F}\boldsymbol{\gamma}^{IK} + \mathbf{C}^{I\top}\mathbf{G}[\mathbf{C}^K]\right] \tag{S3}$$

$$N_{IK} := \langle 0_I|0_K\rangle = c_0^I c_0^K + \mathrm{Tr}[\mathbf{C}^{I\top}\mathbf{C}^K] \tag{S4}$$

representing the coupling between the $I$th and $K$th CIS states. We have used the following intermediates:

$$(\mathbf{C}^I)_{pq} = c_{ai}^I \delta_{pa}\delta_{iq} \tag{S5}$$

$$(\boldsymbol{\gamma}^{IK})_{pq} = \left(c_0^I\mathbf{C}^K + c_0^K\mathbf{C}^{I\top} - \mathbf{C}^{I\top}\mathbf{C}^K + \mathbf{C}^K\mathbf{C}^{I\top}\right)_{pq} \tag{S6}$$

and

$$(\mathbf{G}[\mathbf{M}])_{pq} = \langle pr||qs\rangle M_{sr} \tag{S7}$$

which is the Fock-like matrix evaluated with the matrix $\mathbf{M}$ instead of the HF density matrix $\boldsymbol{\rho}$, i.e., $\mathbf{F} \equiv \mathbf{h} + \mathbf{G}[\boldsymbol{\rho}]$ with $\mathbf{h}$ being the one-electron Hamiltonian.

$\mathbf{C}^I$ is the $N \times N$ matrix containing the CIS vector $c_{ai}^I$ in the vo block. Together with $c_0^I$, it is usually orthonormalized such that $N_{IK} = \delta_{IK}$.

### B. One-particle, two-particle, and transition density matrices

The one- and two-particle density matrices (1PDM and 2PDM) of the CIS state $|0_I\rangle$ are the special case of the transition 1PDM and 2PDM, expressed as

$$P_{qp}^{IK} = \langle 0_I|a_p^\dagger a_q|0_K\rangle = N_{IK}(\boldsymbol{\rho})_{pq} + (\boldsymbol{\gamma}^{IK})_{pq} \tag{S8}$$

$$P_{qp,sr}^{IK} = \langle 0_I|a_p^\dagger a_q^\dagger a_s a_r|0_K\rangle = \mathcal{P}(pq)\mathcal{P}(rs)\left(\frac{1}{2}N_{IK}(\boldsymbol{\rho})_{rp}(\boldsymbol{\rho})_{sq} + (\boldsymbol{\gamma}^{IK})_{rp}(\boldsymbol{\rho})_{sq} + (\mathbf{C}^K)_{rp}(\mathbf{C}^{I\top})_{sq}\right) \tag{S9}$$

where $\mathcal{P}(pq)$ is the anti-symmetrizer. The 1PDM and 2PDM are the diagonals of the transition density matrices ($I = K$). Obviously, the CIS energy is given by

$$E_{0,I} = \sum_{pq} h_{pq} P_{qp}^{II} + \frac{1}{4}\sum_{pqrs}\langle pq||rs\rangle P_{qp,sr}^{II} \tag{S10}$$

In the following, we will omit $I$ and $K$ to implicitly indicate the diagonal ($I = K$), unless otherwise noted.

## C. Gradients

### 1. CI gradients ${}^{\mathrm{c}}g_\mu$

The CIS energy is variationally minimized by optimizing the CI coefficients. This results in the following gradient:

$$ {}^{\mathrm{c}}g_\mu = \langle \Phi_\mu | (\hat{H} - E_0) | 0 \rangle + \langle 0 | (\hat{H} - E_0) | \Phi_\mu \rangle \tag{S11} $$

and

$$ \langle \Phi_0 | (\hat{H} - E_0) | 0 \rangle = (E_{\mathrm{HF}} - E_0) c_0 + \mathrm{Tr}[\mathbf{FC}] \tag{S12} $$

$$ \langle \Phi_i^a | (\hat{H} - E_0) | 0 \rangle = \Big[ (E_{\mathrm{HF}} - E_0)\mathbf{C} + c_0 \mathbf{F} + \mathbf{FC} - \mathbf{CF} + \mathbf{G}[\mathbf{C}] \Big]_{ai} \tag{S13} $$

and

$$ \langle 0 | (\hat{H} - E_0) | \Phi_0 \rangle = (E_{\mathrm{HF}} - E_0) c_0 + \mathrm{Tr}[\mathbf{FC}^\top] \tag{S14} $$

$$ \langle 0 | (\hat{H} - E_0) | \Phi_i^a \rangle = \Big[ (E_{\mathrm{HF}} - E_0)\mathbf{C}^\top + c_0 \mathbf{F} + \mathbf{C}^\top \mathbf{F} - \mathbf{FC}^\top + (\mathbf{G}[\mathbf{C}^\top]) \Big]_{ia} \tag{S15} $$

where it should be noted that $\mathbf{G}[\mathbf{C}^\top] \equiv (\mathbf{G}[\mathbf{C}])^\top$.

Eqs.(S14) and (S15) are the complex conjugates of Eqs.(S12) and (S13) and therefore do not have to be explicitly computed. However, they yield different contributions to the relaxed density matrices when the derivatives are taken.

### 2. Orbital gradients ${}^{\mathrm{o}}g_{ai}$

The gradient can be defined as

$$ {}^{\mathrm{o}}g_{ai} = \langle 0 | \Big[ \hat{E}^-_{ai}, (\hat{H} - E_0) \Big] | 0 \rangle \tag{S16} $$

To evaluate this term, we decompose it to different contributions:

$$ {}^{\mathrm{o}}g_{ai} = L_{ia} - L_{ai} - \bar{L}_{ia} + \bar{L}_{ai} \tag{S17} $$

with

$$ L^{I^*K}_{pq} := \langle 0_I | \hat{E}_{qp} (\hat{H} - E_{0,I}) | 0_K \rangle \tag{S18} $$

$$ \bar{L}^{I^*K}_{pq} := \langle 0_I | (\hat{H} - E_{0,I}) \hat{E}_{qp} | 0_K \rangle = (L^{KI^*}_{qp})^* \tag{S19} $$

where the star indicates the state for which the energy $E_{0,I}$ is used. Again, $L_{pq}$ is shorthand for $L^{I^*I}_{pq}$. Using the hole density matrix $\boldsymbol{\eta}$,

$$ \boldsymbol{\eta} = \mathbf{I} - \boldsymbol{\rho}, \tag{S20} $$

they are expressed as

$$ \begin{aligned} \mathbf{L}^{I^*K} = {} & \boldsymbol{\gamma}^{IK}(E_{\mathrm{HF}} - E_{0,I}) - \boldsymbol{\gamma}^{IK}\mathbf{F}\boldsymbol{\rho} + \boldsymbol{\eta}\mathbf{F}\boldsymbol{\gamma}^{IK} + \boldsymbol{\eta}\mathbf{F}\boldsymbol{\rho} N_{IK} + \boldsymbol{\eta}\mathbf{G}[\boldsymbol{\gamma}^{IK}]\boldsymbol{\rho} \\ & + \mathbf{C}^{I\top}\mathrm{Tr}[\mathbf{FC}^K] + \mathbf{C}^K \mathrm{Tr}[\mathbf{FC}^{I\top}] - \mathbf{C}^{I\top}\mathbf{FC}^K - \mathbf{C}^K\mathbf{FC}^{I\top} \\ & - \mathbf{C}^{I\top}\mathbf{G}[\mathbf{C}^K]\boldsymbol{\rho} - \mathbf{C}^K\mathbf{G}[\mathbf{C}^{I\top}]\boldsymbol{\rho} + \boldsymbol{\eta}\mathbf{G}[\mathbf{C}^K]\mathbf{C}^{I\top} + \boldsymbol{\eta}\mathbf{G}[\mathbf{C}^{I\top}]\mathbf{C}^K \end{aligned} \tag{S21} $$

$$ \begin{aligned} \bar{\mathbf{L}}^{I^*K} = {} & \boldsymbol{\gamma}^{IK}(E_{\mathrm{HF}} - E_0) - \boldsymbol{\rho}\mathbf{F}\boldsymbol{\gamma}^{IK} + \boldsymbol{\gamma}^{IK}\mathbf{F}\boldsymbol{\eta} + \boldsymbol{\rho}\mathbf{F}\boldsymbol{\eta} N_{IK} + \boldsymbol{\rho}\mathbf{G}[\boldsymbol{\gamma}^{IK}]\boldsymbol{\eta} \\ & + \mathbf{C}^{I\top}\mathrm{Tr}[\mathbf{FC}^K] + \mathbf{C}^K \mathrm{Tr}[\mathbf{FC}^{I\top}] - \mathbf{C}^{I\top}\mathbf{FC}^K - \mathbf{C}^K\mathbf{FC}^{I\top} \\ & + \mathbf{C}^{I\top}\mathbf{G}[\mathbf{C}^K]\boldsymbol{\eta} + \mathbf{C}^K\mathbf{G}[\mathbf{C}^{I\top}]\boldsymbol{\eta} - \boldsymbol{\rho}\mathbf{G}[\mathbf{C}^K]\mathbf{C}^{I\top} - \boldsymbol{\rho}\mathbf{G}[\mathbf{C}^{I\top}]\mathbf{C}^K \end{aligned} \tag{S22} $$

It should be apparent that for a converged CIS state where ${}^{\mathrm{c}}g_\mu = 0$, only $L_{ai}$ (and $\bar{L}_{ia}$) are nonzero.

### D. CIS Hessian

In order to facilitate computation, we employ the Davidson algorithm to diagonalize the augmented Hessian. For the augmented Hessian, a trial vector $\mathbf{x} = \begin{pmatrix} x_0 & {}^{\mathrm{o}}\mathbf{x} & {}^{\mathrm{c}}\mathbf{x} \end{pmatrix}^\top$ is multiplied by ${}^{\mathrm{oo}}\mathbf{H}$, ${}^{\mathrm{oc}}\mathbf{H}$, and ${}^{\mathrm{cc}}\mathbf{H}$ to obtain the so-called sigma-vectors

$$ {}^{\mathrm{o}}\sigma_{ai} = {}^{\mathrm{o}}g_{ai}x_0 + \sum_{bj} {}^{\mathrm{oo}}H_{ai,bj}\,{}^{\mathrm{o}}x_{bj} + \sum_{\mu} {}^{\mathrm{oc}}H_{ai,\mu}\,{}^{\mathrm{c}}x_{\mu} \tag{S23} $$

$$ {}^{\mathrm{c}}\sigma_{\mu} = {}^{\mathrm{c}}g_{\mu}x_0 + \sum_{ai} {}^{\mathrm{co}}H_{\mu,ai}\,{}^{\mathrm{o}}x_{ai} + \sum_{\nu} {}^{\mathrm{cc}}H_{\mu,\nu}\,{}^{\mathrm{c}}x_{\nu} \tag{S24} $$

Although occupied-occupied and virtual-virtual orbital rotations are redundant, in our derivation, we deliberately use the full spin orbitals $p, q, r, s$, to make use of anti-symmetry of quantities as well as to keep the simplicity of equations as much as possible in terms of matrix-matrix multiplications. To arrive at the final working equations of (S23) and (S24) where only occupied-virtual rotations are taken into account, one only needs to replace the indices $p, q$ with $a, i$.

We will not show the matrix elements of the Hessian explicitly, because they can be easily deduced from the sigma-vectors.

#### 1. *Contraction of* ${}^{\mathrm{oo}}H_{ai,bj}$ *with* ${}^{\mathrm{o}}x_{bj}$

Let us first define our notation. We write the orbital Hessian of a CIS state as

$$ \begin{aligned} {}^{\mathrm{oo}}H_{pq,rs} := {} & \frac{1}{2}\langle 0|\left[\hat{E}^-_{pq}, \left[\hat{E}^-_{rs}, (\hat{H}-E_0)\right]\right]|0\rangle + \frac{1}{2}\langle 0|\left[\hat{E}^-_{rs}, \left[\hat{E}^-_{pq}, (\hat{H}-E_0)\right]\right]|0\rangle \\ & - {}^{\mathrm{o}}g_{pq}\langle 0|\left[\hat{E}^-_{rs},\right]|0\rangle \end{aligned} \tag{S25} $$

To evaluate this, we define

$$ A_{qp,rs} = \langle 0|\hat{E}_{pq}(\hat{H}-E_0)\hat{E}_{rs}|0\rangle = \langle 0|\hat{E}_{sr}(\hat{H}-E_0)\hat{E}_{qp}|0\rangle^* = A^*_{rs,qp} \tag{S26} $$

$$ B_{pq,rs} = \langle 0|(\hat{H}-E_0)\hat{E}_{pq}\hat{E}_{rs}|0\rangle = \langle 0|\hat{E}_{sr}\hat{E}_{qp}(\hat{H}-E_0)|0\rangle^* \tag{S27} $$

where $\langle 0|0\rangle = N$ is normalized to unity. Using these, it is easy to show that the second derivative of the CIS energy is

$$ {}^{\mathrm{oo}}H_{pq,rs} = \mathcal{P}(pq)\mathcal{P}(rs)\left( A^*_{pq,rs} + A_{pq,rs} + \frac{1}{2}B_{pq,rs} + \frac{1}{2}B_{rs,pq} + \frac{1}{2}B^*_{pq,rs} + \frac{1}{2}B^*_{rs,pq} \right). \tag{S28} $$

and, for real orbitals,

$$ {}^{\mathrm{oo}}H_{pq,rs} = \mathcal{P}(pq)\mathcal{P}(rs)\left( 2A_{pq,rs} + B_{pq,rs} + B_{rs,pq} \right). \tag{S29} $$

Furthermore, since

$$ \hat{E}_{rs}\hat{E}_{pq} = \hat{E}_{pq}\hat{E}_{rs} - \hat{E}_{ps}\delta_{qr} + \hat{E}_{rq}\delta_{ps}, \tag{S30} $$

and thus

$$ B_{rs,pq} = B_{pq,rs} - L_{sp}\delta_{qr} + L_{qr}\delta_{ps}, \tag{S31} $$

we have

$$ {}^{\mathrm{oo}}H_{pq,rs} = \mathcal{P}(pq)\mathcal{P}(rs)\left( 2A_{pq,rs} + 2B_{pq,rs} - L_{sp}\delta_{qr} + L_{qr}\delta_{ps} \right). \tag{S32} $$

Using

$$ \tilde{A}_{qp,rs} = \langle 0|\left[\hat{E}_{pq}, (\hat{H}-E_0)\right]\hat{E}_{rs}|0\rangle \tag{S33} $$

we can express $\mathbf{A}$ as

$$A_{qp,rs} = \tilde{A}_{qp,rs} + B_{pq,rs} \tag{S34}$$

Now we derive the sigma-vectors $\mathbf{A}^{\mathrm{o}}\mathbf{x}$ and $\mathbf{B}^{\mathrm{o}}\mathbf{x}$. For convenience, we define the following intermediates,

$$\mathbf{Q}[^{\mathrm{o}}\mathbf{x}] = \boldsymbol{\eta}^{\mathrm{o}}\mathbf{x}\boldsymbol{\gamma} - \boldsymbol{\gamma}^{\mathrm{o}}\mathbf{x}\boldsymbol{\rho} - \mathbf{C}^{\top\mathrm{o}}\mathbf{x}\mathbf{C} - \mathbf{C}^{\mathrm{o}}\mathbf{x}\mathbf{C}^{\top} + \mathrm{Tr}[\mathbf{C}^{\top\mathrm{o}}\mathbf{x}]\mathbf{C} + \mathrm{Tr}[\mathbf{C}^{\mathrm{o}}\mathbf{x}]\mathbf{C}^{\top} \tag{S35}$$

$$\bar{\boldsymbol{\mathcal{D}}}[^{\mathrm{o}}\mathbf{x}] = \boldsymbol{\eta}^{\mathrm{o}}\mathbf{x}\mathbf{C}^{\top} - \mathbf{C}^{\top\mathrm{o}}\mathbf{x}\boldsymbol{\rho} \tag{S36}$$

$$^{\mathrm{o}}\mathbf{X}[^{\mathrm{o}}\mathbf{x}] = \boldsymbol{\eta}^{\mathrm{o}}\mathbf{x}\boldsymbol{\rho} \tag{S37}$$

and let

$$\boldsymbol{\Omega}^{I} = \mathbf{Q}[^{\mathrm{o}}\mathbf{x}] + {}^{\mathrm{o}}\mathbf{X}N + \boldsymbol{\rho}\mathrm{Tr}[\boldsymbol{\gamma}^{\mathrm{o}}\mathbf{x}] \tag{S38}$$

Then, after simple algebra,

$$\begin{aligned}\sum_{rs}(\tilde{\mathbf{A}})_{qp,rs}{}^{\mathrm{o}}\tilde{x}_{rs} = \Bigg(&\big[\mathbf{F},\boldsymbol{\Omega}^{I}\big] + \big[\mathbf{G}[\boldsymbol{\Omega}^{I}],\boldsymbol{\rho}\big] - [\mathbf{F},\boldsymbol{\rho}]\,\mathrm{Tr}[\mathbf{P}^{\mathrm{o}}\mathbf{x}] + \big[\mathbf{G}[\mathbf{C}],\bar{\boldsymbol{\mathcal{D}}}\big] \\ &+ \big[\mathbf{G}[\bar{\boldsymbol{\mathcal{D}}}],\mathbf{C}\big] + [\mathbf{G}[\gamma],{}^{\mathrm{o}}\mathbf{X}] + [\mathbf{G}[^{\mathrm{o}}\mathbf{X}],\gamma]\Bigg)_{qp}\end{aligned} \tag{S39}$$

$$\begin{aligned}\sum_{rs}(\mathbf{B})_{pq,rs}{}^{\mathrm{o}}x_{rs} = \Bigg(&\boldsymbol{\eta}^{\mathrm{o}}\mathbf{x}\mathbf{L} - \mathbf{L}^{\mathrm{o}}\mathbf{x}\boldsymbol{\rho} + \boldsymbol{\rho}\mathrm{Tr}[\mathbf{L}^{\mathrm{o}}\mathbf{x}] \\ &+ (E_{\mathrm{HF}} - E_0)\Big(\mathbf{Q} - \boldsymbol{\eta}^{\mathrm{o}}\mathbf{x}\boldsymbol{\gamma} + \boldsymbol{\gamma}^{\mathrm{o}}\mathbf{x}\boldsymbol{\rho}\Big) + \Big(\mathbf{Q} - \boldsymbol{\eta}^{\mathrm{o}}\mathbf{x}\boldsymbol{\gamma}\Big)\mathbf{F}\boldsymbol{\eta} - \boldsymbol{\rho}\mathbf{F}\Big(\mathbf{Q} + \boldsymbol{\gamma}^{\mathrm{o}}\mathbf{x}\boldsymbol{\rho}\Big) \\ &+ \mathbf{C}(^{\mathrm{o}}\mathbf{x}\boldsymbol{\rho}\mathbf{F} - \mathbf{F}\boldsymbol{\eta}^{\mathrm{o}}\mathbf{x})\mathbf{C}^{\top} + \mathbf{C}^{\top}(^{\mathrm{o}}\mathbf{x}\boldsymbol{\rho}\mathbf{F} - \mathbf{F}\boldsymbol{\eta}^{\mathrm{o}}\mathbf{x})\mathbf{C} + \boldsymbol{\rho}\mathbf{F}\boldsymbol{\eta}\mathrm{Tr}[\boldsymbol{\gamma}^{\mathrm{o}}\mathbf{x}] \\ &- \boldsymbol{\rho}\mathbf{G}[\mathbf{C}]\boldsymbol{\eta}^{\mathrm{o}}\mathbf{x}\mathbf{C}^{\top} - \mathbf{C}^{\top\mathrm{o}}\mathbf{x}\boldsymbol{\rho}\mathbf{G}[\mathbf{C}]\boldsymbol{\eta} - \boldsymbol{\rho}\mathbf{G}[\mathbf{C}^{\top}]\boldsymbol{\eta}^{\mathrm{o}}\mathbf{x}\mathbf{C} - \mathbf{C}^{\mathrm{o}}\mathbf{x}\boldsymbol{\rho}\mathbf{G}[\mathbf{C}^{\top}]\boldsymbol{\eta} \\ &+ \mathbf{C}\mathrm{Tr}[\mathbf{F}\bar{\boldsymbol{\mathcal{D}}}] + \mathbf{C}\mathbf{G}[\bar{\boldsymbol{\mathcal{D}}}]\boldsymbol{\eta} - \boldsymbol{\rho}\mathbf{G}[\bar{\boldsymbol{\mathcal{D}}}]\mathbf{C} \\ &+ \mathbf{C}\mathrm{Tr}\Big(\mathbf{G}[^{\mathrm{o}}\mathbf{X}]\mathbf{C}^{\top}\Big) - \mathbf{C}\mathbf{G}[^{\mathrm{o}}\mathbf{X}]\mathbf{C}^{\top} + \mathbf{C}^{\top}\mathrm{Tr}\Big(\mathbf{G}[\mathbf{X}]\mathbf{C}\Big) - \mathbf{C}^{\top}\mathbf{G}[\mathbf{X}]\mathbf{C} \\ &+ \boldsymbol{\gamma}\mathrm{Tr}[\mathbf{F}\mathbf{X}] + \mathbf{P}\mathbf{G}[\mathbf{X}]\boldsymbol{\eta} - \boldsymbol{\rho}\mathbf{G}[^{\mathrm{o}}\mathbf{X}]\boldsymbol{\gamma} + \boldsymbol{\rho}\mathbf{G}[\mathbf{Q}]\boldsymbol{\eta}\Bigg)_{qp}\end{aligned} \tag{S40}$$

With these, one can evaluate the contraction of $\sum_{bj}{}^{\mathrm{oo}}H_{ai,bj}{}^{\mathrm{o}}x_{bj}$. Note that, again, the result is very general, and may be further simplified by using the facts that $\mathbf{F}$ is diagonal in HF and that only the vo block is needed. For example, for the restricted HF, the multiplications with $\boldsymbol{\rho}$ and $\boldsymbol{\eta}$ indicate the projection to the occupied and virtual spaces, respectively.

### 2. *Contraction of* ${}^{\mathrm{oc}}H_{ai,\mu}$ *with* ${}^{\mathrm{c}}x_{\mu}$ *and* ${}^{\mathrm{o}}x_{ai}$

We have two types of sigma-vectors. The first one is contracted with the CI trial vector ${}^{\mathrm{c}}\mathbf{x}$. We conveniently define the following quantities:

$$|\mathbf{x}\rangle = \sum_{\mu}{}^{\mathrm{c}}x_{\mu}|\Phi_{\mu}\rangle \tag{S41}$$

and

$$L^{I^*\mathbf{x}}_{pq} = \langle 0_I|\hat{E}_{qp}(\hat{H} - E_{0,I})|\mathbf{x}\rangle \tag{S42}$$

$$L^{\mathbf{x}I^*}_{pq} = \langle \mathbf{x}|\hat{E}_{qp}(\hat{H} - E_{0,I})|0_I\rangle \tag{S43}$$

$$\bar{L}^{I^*\mathbf{x}}_{pq} = \langle 0_I|(\hat{H} - E_{0,I})\hat{E}_{qp}|\mathbf{x}\rangle = (L^{\mathbf{x}I^*}_{qp})^* \tag{S44}$$

$$\bar{L}^{\mathbf{x}I^*}_{pq} = \langle \mathbf{x}|(\hat{H} - E_{0,I})\hat{E}_{qp}|0_I\rangle = (L^{I^*\mathbf{x}}_{qp})^* \tag{S45}$$

Note that $L_{pq}^{I^*\mathbf{x}}$ ($L_{pq}^{\mathbf{x}I^*}$) can be obtained in exactly the same manner as $L_{pq}$ (using Eq.(S21)), by simply replacing $\mathbf{C}$ ($\mathbf{C}^\top$) by ${}^{\mathrm{c}}\mathbf{x}$ while $\mathbf{C}^\top$ ($\mathbf{C}$) is kept unchanged. This then requires the new two-electron contractions, $\mathbf{G}[\boldsymbol{\gamma}^{I\mathbf{x}}]$ and $\mathbf{G}[{}^{\mathrm{c}}\mathbf{x}]$ where

$$\boldsymbol{\gamma}^{I\mathbf{x}} = c_0^{I\,\mathrm{c}}\mathbf{x} + {}^{\mathrm{c}}x_0\mathbf{C}^{I\top} - \mathbf{C}^{I\top\mathrm{c}}\mathbf{x} + {}^{\mathrm{c}}\mathbf{x}\mathbf{C}^{I\top} \tag{S46}$$

Then, the sigma-vector contracted with ${}^{\mathrm{c}}x_\mu$ is

$$\sum_\mu {}^{\mathrm{oc}}H_{pq,\mu}{}^{\mathrm{c}}x_\mu = 2\mathcal{P}(pq)\Big(L_{qp}^{I^*\mathbf{x}} + L_{qp}^{\mathbf{x}I^*} - 2L_{qp}^{I^*I}\sum_\nu (c_\nu^{I\,\mathrm{c}}x_\nu)\Big) \tag{S47}$$

where we have used the fact all the quantities are real.

The second sigma-vector is the one contracted with ${}^{\mathrm{o}}x_{ai}$.

$$\sum_{pq} {}^{\mathrm{co}}H_{\mu,pq}{}^{\mathrm{o}}x_{pq} = -4\sum_\mu \left(\langle\Phi_\mu|(\hat{H}-E_0)\hat{E}_{pq}|0\rangle{}^{\mathrm{o}}x_{pq} + \langle 0|(\hat{H}-E_0)\hat{E}_{pq}|\Phi_\mu\rangle{}^{\mathrm{o}}x_{pq} + 2\mathrm{Tr}\left[\mathbf{L}{}^{\mathrm{o}}\mathbf{x}\right]c_\mu\right) \tag{S48}$$

We can extract the matrix elements $\langle\Phi_\mu|(\hat{H}-E_0)\hat{E}_{pq}|0\rangle$ and $\langle 0|(\hat{H}-E_0)\hat{E}_{pq}|\Phi_\mu\rangle$ by taking the derivatives of $L_{qp}$ and $\bar{L}_{qp}$ with respect to the CI coefficients $c_\mu$. The result is

$$\begin{aligned}\sum_{pq}\langle\Phi_0|(\hat{H}-E_0)\hat{E}_{pq}|0\rangle{}^{\mathrm{o}}x_{pq} = {} & \mathrm{Tr}[\mathbf{C}{}^{\mathrm{o}}\mathbf{x}](E_{\mathrm{HF}}-E_0) - \mathrm{Tr}[\mathbf{C}{}^{\mathrm{o}}\mathbf{x}\boldsymbol{\rho}\mathbf{F}] \\ & + \mathrm{Tr}[\mathbf{C}\mathbf{F}\boldsymbol{\eta}{}^{\mathrm{o}}\mathbf{x}] + \mathrm{Tr}[\mathbf{F}{}^{\mathrm{o}}\mathbf{X}]c_0 + \mathrm{Tr}[\mathbf{G}[\mathbf{C}]{}^{\mathrm{o}}\mathbf{X}]\end{aligned} \tag{S49}$$

$$\begin{aligned}\sum_{pq}\langle 0|(\hat{H}-E_0)\hat{E}_{pq}|\Phi_0\rangle{}^{\mathrm{o}}x_{pq} = {} & \mathrm{Tr}[\mathbf{C}^\top{}^{\mathrm{o}}\mathbf{x}](E_{\mathrm{HF}}-E_0) - \mathrm{Tr}[\mathbf{C}^\top{}^{\mathrm{o}}\mathbf{x}\boldsymbol{\rho}\mathbf{F}] \\ & + \mathrm{Tr}[\mathbf{C}^\top\mathbf{F}\boldsymbol{\eta}{}^{\mathrm{o}}\mathbf{x}] + \mathrm{Tr}[\mathbf{F}{}^{\mathrm{o}}\mathbf{X}]c_0 + \mathrm{Tr}[\mathbf{G}[\mathbf{C}^\top]{}^{\mathrm{o}}\mathbf{X}]\end{aligned} \tag{S50}$$

which are symmetric with respect to $\mathbf{C}$ and $\mathbf{C}^\top$. For the projection to singly excited determinants,

$$\begin{aligned}\sum_{pq}\langle\Phi_i^a|(\hat{H}-E_0)\hat{E}_{pq}|0\rangle{}^{\mathrm{o}}x_{pq} = {} & \Big(c_0\mathbf{T} + \mathbf{T}\mathbf{C} - \mathbf{C}\mathbf{T} + \mathrm{Tr}[\mathbf{F}{}^{\mathrm{o}}\mathbf{X}]\mathbf{C} + {}^{\mathrm{o}}\mathbf{x}\mathrm{Tr}[\mathbf{F}\mathbf{C}] - \mathbf{F}\mathbf{C}{}^{\mathrm{o}}\mathbf{x} - {}^{\mathrm{o}}\mathbf{x}\mathbf{C}\mathbf{F} + \mathrm{Tr}[\mathbf{C}{}^{\mathrm{o}}\mathbf{x}]\mathbf{F} \\ & + \mathbf{G}[\mathbf{C}]\boldsymbol{\eta}{}^{\mathrm{o}}\mathbf{x} - {}^{\mathrm{o}}\mathbf{x}\boldsymbol{\rho}\mathbf{G}[\mathbf{C}]\Big)_{ai}\end{aligned} \tag{S51}$$

and

$$\begin{aligned}\sum_{pq}\langle 0|(\hat{H}-E_0)\hat{E}_{pq}|\Phi_k^c\rangle{}^{\mathrm{o}}x_{pq} = {} & \Big(c_0\mathbf{T} + \mathbf{C}^\top\mathbf{T} - \mathbf{T}\mathbf{C}^\top + \mathrm{Tr}[\mathbf{F}{}^{\mathrm{o}}\mathbf{X}]\mathbf{C}^\top + {}^{\mathrm{o}}\mathbf{x}\mathrm{Tr}[\mathbf{F}\mathbf{C}^\top] - {}^{\mathrm{o}}\mathbf{x}\mathbf{C}^\top\mathbf{F} - \mathbf{F}\mathbf{C}^\top{}^{\mathrm{o}}\mathbf{x} + \mathrm{Tr}[\mathbf{C}^\top{}^{\mathrm{o}}\mathbf{x}]\mathbf{F} \\ & + \mathbf{G}[\mathbf{C}^\top]\boldsymbol{\eta}{}^{\mathrm{o}}\mathbf{x} - {}^{\mathrm{o}}\mathbf{x}\boldsymbol{\rho}\mathbf{G}[\mathbf{C}^\top]\Big)_{kc}\end{aligned} \tag{S52}$$

where

$$\mathbf{T} = (E_{\mathrm{HF}}-E_0){}^{\mathrm{o}}\mathbf{x} + \mathbf{F}\boldsymbol{\eta}{}^{\mathrm{o}}\mathbf{x} - {}^{\mathrm{o}}\mathbf{x}\boldsymbol{\rho}\mathbf{F} + \mathbf{G}[{}^{\mathrm{o}}\mathbf{X}] \tag{S53}$$

was introduced to simply the equations.

### 3. Contraction of ${}^{\mathrm{cc}}H_{\mu\nu}$ with ${}^{\mathrm{c}}x_\nu$

Using the shorthand notation Eq.(S41),

$$\sum_\mu {}^{\mathrm{cc}}H_{\mu\nu}{}^{\mathrm{c}}x_\nu = 2\langle\Phi_\mu|(\hat{H}-E_0)|\mathbf{x}\rangle - c_\mu \sum_\nu {}^{\mathrm{c}}g_\nu {}^{\mathrm{c}}x_\nu - {}^{\mathrm{c}}g_\mu \sum_\nu c_\nu {}^{\mathrm{c}}x_\nu \tag{S54}$$

## E. Formation of Fock-like matrices

The above results indicate that, to construct each component of the gradients and the Hessian's sigma-vector, namely, ${}^{\mathrm{o}}\mathbf{g}$, ${}^{\mathrm{c}}\mathbf{g}$, ${}^{\mathrm{oo}}\mathbf{H}{}^{\mathrm{o}}\mathbf{x}$, ${}^{\mathrm{oc}}\mathbf{H}{}^{\mathrm{c}}\mathbf{x}$, ${}^{\mathrm{co}}\mathbf{H}{}^{\mathrm{o}}\mathbf{x}$, and ${}^{\mathrm{cc}}\mathbf{H}{}^{\mathrm{c}}\mathbf{x}$, we need to contract the two-electron integrals with $\mathbf{C}$ and $\boldsymbol{\gamma}$ for the gradients, and $\mathbf{Q}$ (Eq.(S35)), $\bar{\boldsymbol{\mathcal{D}}}$ (Eq.(S36)), ${}^{\mathrm{o}}\mathbf{X}$ (Eq.(S37)), ${}^{\mathrm{c}}\mathbf{x}$, and $\boldsymbol{\gamma}^{I\mathbf{x}}$ (Eq.(S46)), for the sigma-vectors. These are summarized in the table below. All these contractions are only necessary to be performed in a Fock-like manner as $\boldsymbol{G}[\mathbf{M}]$ and thus are at a $O(N^4)$ cost, without the need of the explicit orbital transformation of AO integrals. Moreover, $\mathbf{C}$ and $\boldsymbol{\gamma}$ need to be contracted once. Therefore, at each iteration of the Hessian-based optimization or DCIS relaxation, five Fock-like matrices are constructed.

| Quantity | Necessary contraction |
|---|---|
| ${}^{\mathrm{o}}\mathbf{g}$ | $\mathbf{C}, \boldsymbol{\gamma}$ |
| ${}^{\mathrm{c}}\mathbf{g}$ | $\mathbf{C}$ |
| ${}^{\mathrm{oo}}\mathbf{H}{}^{\mathrm{o}}\mathbf{x}$ | $\boldsymbol{\gamma}, \mathbf{Q}, \bar{\boldsymbol{\mathcal{D}}}, {}^{\mathrm{o}}\mathbf{X}$ |
| ${}^{\mathrm{oc}}\mathbf{H}{}^{\mathrm{c}}\mathbf{x}$ | ${}^{\mathrm{c}}\mathbf{x}, \boldsymbol{\gamma}^{I\mathbf{x}}$ |
| ${}^{\mathrm{co}}\mathbf{H}{}^{\mathrm{o}}\mathbf{x}$ | $\mathbf{C}, {}^{\mathrm{o}}\mathbf{X}$ |
| ${}^{\mathrm{cc}}\mathbf{H}{}^{\mathrm{c}}\mathbf{x}$ | ${}^{\mathrm{c}}\mathbf{x}$ |

# II. Double CIS expressed in many ways

Here, we will provide proof that the different ansätze proposed in the main text result in the same variational space. First, the formal definition of our DCIS wave function is

$$|\Psi_{\mathrm{DCIS}}\rangle = (1-\hat{\kappa})|0\rangle + (1-|0\rangle\langle 0|)\sum_\mu \bar{c}_\mu|\Phi_\mu\rangle \tag{S55}$$

where the parameters $\kappa_{ai}$ and $\bar{c}_\mu$ are to be variationally optimized. By expanding this wave function and sorting it out based on each level of excitations with respect to the HF vacuum,

$$\begin{aligned}
|\Psi_{\mathrm{DCIS}}\rangle &= |0\rangle + \left(\sum_{ai}\kappa_{ai}c_{ai}\right)|\Phi_0\rangle - \sum_{abij}\kappa_{ai}c_{bj}|\Phi_{ij}^{ab}\rangle + \sum_\mu \bar{c}_\mu|\Phi_\mu\rangle - |0\rangle\sum_\mu c_\mu\bar{c}_\mu \\
&= \sum_{ai}c_{ai}|\Phi_i^a\rangle + \left(\sum_{ai}\kappa_{ai}c_{ai}\right)|\Phi_0\rangle - \kappa_{ai}c_{bj}|\Phi_{ij}^{ab}\rangle + \bar{c}_0|\Phi_0\rangle + \sum_{ai}\bar{c}_{ai}|\Phi_i^a\rangle - \left(\sum_{bj}c_{bj}\bar{c}_{bj}\right)\sum_{ai}c_{ai}|\Phi_i^a\rangle \\
&= \bar{c}_0|\Phi_0\rangle + \left(\sum_{ai}\kappa_{ai}c_{ai}\right)|\Phi_0\rangle + \sum_{ai}c_{ai}|\Phi_i^a\rangle - \left(\sum_{bj}c_{bj}\bar{c}_{bj}\right)\sum_{ai}c_{ai}|\Phi_i^a\rangle + \sum_{ai}\bar{c}_{ai}|\Phi_i^a\rangle - \sum_{abij}\kappa_{ai}c_{bj}|\Phi_{ij}^{ab}\rangle \\
&= \left(\bar{c}_0 + \sum_{ai}\kappa_{ai}c_{ai}\right)|\Phi_0\rangle + \sum_{ai}\left(\left(1-\sum_{bj}c_{bj}\bar{c}_{bj}\right)c_{ai} + \bar{c}_{ai}\right)|\Phi_i^a\rangle - \sum_{abij}\kappa_{ai}c_{bj}|\Phi_{ij}^{ab}\rangle
\end{aligned} \tag{S56}$$

Now, we wish to arrange the variational parameters so that $|\Psi_{\mathrm{DCIS}}\rangle$ looks more like the standard Configuration Interaction, without changing its variational space. Since $\bar{c}_0$ only appears in the HF determinant space, the other contribution $\sum_{ai}\kappa_{ai}c_{ai}$ does not play a role. That means, while $\kappa_{ai}$ are varied to maximize the energy lowering contribution from $\kappa_{ai}c_{bj}|\Phi_{ij}^{ab}\rangle$, they do *not* affect the total coefficient of $|\Phi_0\rangle$, because $\bar{c}_0$ can be also varied to cancel the effect. Therefore, we can introduce a single effective coefficient $\bar{d}_0 = \bar{c}_0 + \sum_{ai}\kappa_{ai}c_{ai}$, which can be solely used to parametrize the Hartree-Fock space. This way, any change in $\bar{c}_0$ and $\kappa_{ai}$ can be absorbed in $\bar{d}_0$.

Similarly, the coefficients for $|\Phi_i^a\rangle$ can be replaced by effective CI coefficients $\bar{d}_{ai}$,

$$\bar{d}_{ai} = \left(1 - \sum_{bj} c_{bj}\bar{c}_{bj}\right) c_{ai} + \bar{c}_{ai} \tag{S57}$$

because either $\bar{d}_{ai}$ or $\bar{c}_{ai}$ can entirely parametrize the singles space. Finally, just to make the final result look better, we use $d_{ai} = -\kappa_{ai}$. Putting together, we have

$$|\Psi_{\text{DCIS}}\rangle = \bar{d}_0|\Phi_0\rangle + \sum_{ai} \bar{d}_{ai}|\Phi_i^a\rangle + \sum_{abij} d_{ai}c_{bj}|\Phi_{ij}^{ab}\rangle \tag{S58}$$

which can be also expressed as

$$|\Psi_{\text{DCIS}}\rangle = \sum_{ai} d_{ai}\hat{E}_{ai}|0\rangle + \sum_{\mu} \bar{d}_{\mu}|\Phi_{\mu}\rangle \tag{S59}$$

### A. Proof that internally-contracted CIS is equivalent to DCIS

The parameterization of the internally-contracted CIS,

$$|\Psi\rangle = \sum_{pq} t_{pq}\hat{E}_{pq}|0\rangle \tag{S60}$$

has a significant number of redundancies. Explicitly written, the ansatz is expressed as

$$|\Psi\rangle = \left(\sum_{ai} t_{ia}c_{ai}\right)|\Phi_0\rangle + \sum_{ai}\left(\left(\sum_k t_{kk}\right)c_{ai} + c_0 t_{ai} + \sum_c t_{ac}c_{ci} - \sum_k c_{ak}t_{ki}\right)|\Phi_i^a\rangle + \sum_{aibj} t_{ai}c_{bj}|\Phi_{ij}^{ab}\rangle \tag{S61}$$

Noting that the ov block $\{t_{ia}\}$ appears in the form of summation $\bar{d}_0 = \sum_{ai} t_{ia}c_{ai}$, they are redundant except for one because $\bar{d}_0$ can be regarded as a single variational parameter instead of $\{t_{ia}\}$. Namely, if we define $N_{\text{vo}}$ as the number of the parameters $\{t_{ia}\}$, the dimension of the redundancy due to the ov block is $N_{\text{vo}} - 1$.

The vo block $\{t_{bj}\}$ is free of redundancy, as they specify the weights of doubly excited configuration terms uniquely, i.e., the last term of Eq. (S61). Therefore, they exactly correspond to $\{d_{bj}\}$ of Eq. (S59).

Other blocks, $\{t_{bc}\}, \{t_{jk}\}$ also contain redundancies, as they simply play a role of "dressing" the effective singles' coefficients $\bar{d}_{ai}$ for $|\Phi_i^a\rangle$,

$$\bar{d}_{ai} = \left(\sum_k t_{kk}\right)c_{ai} + \sum_c t_{ac}c_{ci} - \sum_k c_{ak}t_{ki} \tag{S62}$$

Note that any dressed coefficients $\{\bar{d}_{ai}\}$ can be constructed from the contractions of $\{t_{bc}\}, \{t_{jk}\}$ with the fixed $\{c_{ai}\}$, as the total number of the latter variational set $(N_{\text{oo}} + N_{\text{vv}})$ is always larger than that of the former, $N_{\text{vo}}$. Hence, the dimension of the potential redundancy is $N_{\text{oo}} + N_{\text{vv}} - N_{\text{vo}}$.

Overall, the number of the redundancies in the internally-contracted parametrization is $N_{\text{oo}} + N_{\text{vv}} - 1$, out of a total of $N_{\text{oo}} + 2N_{\text{ov}} + N_{\text{vv}}$ parameters. This means that there are $1 + 2N_{ov}$ non-redundant parameters, the same number as that for our DCIS ansatz, as expected.

We have numerically confirmed that the obtained energy spectrum of the internally-contracted CIS is identical to that of DCIS (by performing full diagonalization of the entire Hamiltonian matrix). However, the significant number of redundancies introduced in the ansatz Eq.(S59) poses a numerical challenge in its variational optimization with the standard iterative eigensolver such as the Davidson algorithm. In practice, during the iterative update, the norms of eigenvectors become divergent, although the wavefunction norm $\langle\Psi_{\text{DCIS}}|\Psi_{\text{DCIS}}\rangle$ is kept unity.

## III. Summary of benchmark results

### A. Excitation energy

TABLE S1: Summary of charge transfer excitations.

| Molecule | State (CIS #) | Main MO | CIS $\|^{\circ}g\|$ | Excitation energy (eV) Reference[a] | CIS | ooCIS | DCIS[b] | DCIS[c] | Total energy (a.u.) HF | CIS | DCIS ($S_0$) | DCIS ($S_n$) |
|---|---|---|---|---|---|---|---|---|---|---|---|---|
| **1** Aminobenzonitrile | $A_1$ ($S_2$) | (31-32) | 0.065 | 5.26 | 5.73 | 5.66 | 5.65 | 5.93 | -377.596158 | -377.385445 | -377.606481 | -377.388686 |
| **2** Aniline | $A_1$ ($S_2$) | (25-29) | 0.053 | 5.87 | 6.11 | 6.06 | 6.06 | 6.31 | -285.830849 | -285.606197 | -285.840269 | -285.608202 |
| **3** Azulene | $A_1$ ($S_2$) | (34-36) | 0.072 | 3.89 | 3.99 | 3.89 | 3.76 | 4.02 | -383.406356 | -383.259616 | -383.415951 | -383.268161 |
| | $B_2$ ($S_3$) | (33-36) | 0.097 | 4.55 | 5.54 | 5.36 | 5.20 | 5.54 | | -383.202615 | -383.419080 | -383.215325 |
| **4** Benzonitrile | $A_2$ ($S_3$) | (25-28) | 0.106 | 7.10 | 6.89 | 6.73 | 6.57 | 6.86 | -322.540364 | -322.287040 | -322.551115 | -322.299017 |
| **5** Benzothiadiazole | $B_2$ ($S_1$) | (35-36) | 0.093 | 4.37 | 4.68 | 4.49 | 4.32 | 4.65 | -736.060545 | -735.888669 | -736.072654 | -735.901893 |
| **6** DMABN | $A_1$ ($S_2$) | (39-40) | 0.073 | 4.94 | 5.60 | 5.52 | 5.49 | 5.77 | -455.668731 | -455.462802 | -455.678723 | -455.466855 |
| **7** Dimethylaniline | $B_2$ ($S_1$) | (33-34) | 0.101 | 4.47 | 5.63 | 5.48 | 5.37 | 5.57 | -363.902920 | -363.696109 | -363.910317 | -363.705544 |
| | $A_1$ ($S_2$) | (33-36) | 0.059 | 5.54 | 6.02 | 5.97 | 5.57 | 5.83 | | -363.681538 | -363.912177 | -363.698044 |
| **8** Dipeptide | $A''$ ($S_{24}$) | (33-39) | 0.197 | 8.15 | 11.76 | 11.18 | 10.33 | 10.35 | -453.988444 | -453.556448 | -453.989282 | -453.608788 |
| **9** $\beta$-Dipeptide | $A'$ ($S_{13}$) | (39-43, 38-43) | 0.257 | 8.51 | 10.79 | 9.74 | 9.22 | 9.24 | -493.030362 | -492.633951 | -493.031008 | -492.691613 |
| | $A''$ ($S_{46}$) | (37-43, 37-46) | 0.290 | 8.90 | 12.62 | 11.27 | 10.05 | 10.06 | | -492.566758 | -493.030638 | -492.660929 |
| **10** Hydrogen Chloride | $\Pi_b$ ($S_{1/2}$) | (8/9-10) | 0.178 | 8.10 | 8.58 | 8.06 | 7.63 | 7.70 | -460.106811 | -459.791488 | -460.109622 | -459.826509 |
| **11** Nitroaniline | $A_1$ ($S_1$) | (36-37) | 0.138 | 4.57 | 5.45 | 5.16 | 4.97 | 5.22 | -489.382673 | -489.182316 | -489.391666 | -489.199874 |
| **12** Nitrobenzene | $A_1$ ($S_2$) | (31-33) | 0.106 | 5.57 | 5.87 | 5.60 | 5.46 | 5.64 | -434.324492 | -434.108928 | -434.331190 | -434.123816 |
| **13** NDMA | $A_1$ ($S_1$) | (44-45) | 0.138 | 4.28 | 5.29 | 5.00 | 4.81 | 5.05 | -567.454966 | -567.260624 | -567.463625 | -567.278171 |
| **14** Nitropyridine N-Oxide | $A_1$ ($S_1$) | (36-37) | 0.152 | 4.24 | 4.95 | 4.64 | 4.30 | 4.72 | -525.125260 | -524.943509 | -525.140802 | -524.967306 |
| **15** N-Phenylpyrrole | $B_2$ ($S_3$) | (37-39) | 0.122 | 5.53 | 6.22 | 5.98 | 5.84 | 6.14 | -438.494562 | -438.265993 | -438.505580 | -438.279994 |
| | $A_1$ ($S_5$) | (37-40) | 0.174 | 6.04 | 7.72 | 7.09 | 6.61 | 6.80 | | -438.210909 | -438.501340 | -438.251470 |
| **16** Phthalazine | $A_2$ ($S_4$) | (32-35, 32-39) | 0.206 | 3.93 | 5.70 | 5.02 | 4.63 | 4.79 | -415.436123 | -415.226582 | -415.442188 | -415.266086 |
| | $B_1$ ($S_3$) | (32-36) | 0.163 | 4.34 | 5.63 | 5.20 | 4.88 | 5.09 | | -415.229066 | -415.443711 | -415.256814 |
| **17** Quinoxaline | $B_2$ ($S_2$) | (34-35) | 0.092 | 4.74 | 5.22 | 5.05 | 4.87 | 5.15 | -415.469433 | -415.277675 | -415.479542 | -415.290297 |
| | $A_1$ ($S_5$) | (34-36, 33-38) | 0.111 | 5.75 | 6.88 | 6.62 | 6.52 | 6.84 | | -415.216484 | -415.481075 | -415.229835 |
| | $B_1$ ($S_{14}$) | (32-38) | 0.112 | 6.33 | 8.85 | 8.61 | 8.40 | 8.46 | | -415.144124 | -415.471619 | -415.160556 |
| **18** Twisted-DMABN | $A_2$ ($S_3$) | (38-40) | 0.313 | 4.17 | 6.19 | 4.78 | 4.08 | 4.12 | -455.654023 | -455.426552 | -455.655256 | -455.503954 |
| | $B_1$ ($S_7$) | (38-41) | 0.332 | 4.84 | 7.44 | 5.72 | 4.88 | 4.91 | | -455.380483 | -455.655125 | -455.474567 |
| **19** Twisted-PP | $B_2$ ($S_5$) | (38-40) | 0.290 | 5.73 | 7.37 | 5.80 | 5.30 | 5.33 | -438.496006 | -438.225322 | -438.497042 | -438.301197 |
| | $A_1$ ($S_8$) | (38-39) | 0.108 | 5.82 | 7.82 | 7.55 | 7.55 | 7.81 | | -438.208729 | -438.505620 | -438.218555 |
| | $A_2$ ($S_7$) | (37-40) | 0.250 | 6.04 | 7.77 | 6.73 | 6.31 | 6.35 | | -438.210313 | -438.497518 | -438.264257 |
| | $B_1$ ($S_{12}$) | (37-39) | 0.242 | 6.28 | 8.26 | 7.23 | 6.88 | 6.94 | | -438.192574 | -438.498298 | -438.243303 |

[a] Taken from Ref.[1].
[b] HF $S_0$.
[c] DCIS $S_0$.

### B. Potential energy

TABLE S2: Potential energy of hydrogen fluoride computed with a 6-31G basis.

| $R_{\mathrm{H-F}}$ (Å) | FCI | HF | DCIS | SFCIS |
|---|---|---|---|---|
| 0.70 | −100.005489 | −99.885615 | −99.887628 | −99.837258 |
| 0.80 | −100.087139 | −99.961476 | −99.965965 | −99.929344 |
| 0.90 | −100.114251 | −99.982920 | −99.991268 | −99.968110 |
| 0.95 | −100.116698 | −99.982548 | −99.993338 | −99.975875 |
| 1.00 | −100.114621 | −99.977637 | −99.991183 | −99.978530 |
| 1.10 | −100.102115 | −99.959321 | −99.979199 | −99.973777 |
| 1.20 | −100.083938 | −99.934995 | −99.962094 | −99.961640 |
| 1.40 | −100.044285 | −99.881379 | −99.924976 | −99.931418 |
| 1.60 | −100.009752 | −99.829908 | −99.892730 | −99.904706 |
| 1.80 | −99.984078 | −99.784062 | −99.869141 | −99.885552 |
| 2.00 | −99.967201 | −99.744586 | −99.854233 | −99.873476 |
| 2.10 | −99.961487 | −99.727167 | −99.849413 | −99.869483 |
| 2.20 | −99.957183 | −99.711192 | −99.845906 | −99.866502 |
| 2.40 | −99.951656 | −99.683182 | −99.841624 | −99.862704 |
| 2.60 | −99.948741 | −99.659800 | −99.839485 | −99.860738 |
| 2.80 | −99.947238 | −99.640372 | −99.838365 | −99.859791 |
| 3.00 | −99.946465 | −99.624323 | −99.837694 | −99.859387 |
| 3.20 | −99.946065 | −99.611147 | −99.837221 | −99.859230 |
| 3.40 | −99.945857 | −99.600387 | −99.836850 | −99.859162 |
| 3.60 | −99.945751 | −99.591626 | −99.836546 | −99.859128 |
| 3.80 | −99.945698 | −99.584491 | −99.836295 | −99.859110 |
| 4.00 | −99.945673 | −99.578652 | −99.836085 | −99.859100 |

TABLE S3: Potential energy of diatomic fluoride computed with a 6-31G basis.

| $R_{\mathrm{F-F}}$ (Å) | FCI[a] | HF | DCIS | SFCIS |
|---|---|---|---|---|
| 1.0 | −198.548314 | −198.333080 | −198.338893 | −198.340641 |
| 1.1 | −198.733266 | −198.503076 | −198.518838 | −198.522162 |
| 1.2 | −198.836369 | −198.591745 | −198.619496 | −198.625062 |
| 1.4 | −198.919306 | −198.645963 | −198.699979 | −198.714195 |
| 1.6 | −198.929109 | −198.624352 | −198.707493 | −198.733884 |
| 1.8 | −198.918136 | −198.577976 | −198.694423 | −198.732053 |
| 2.0 | −198.906826 | −198.529095 | −198.682143 | −198.727009 |
| 2.1 | −198.902760 | −198.506457 | −198.678042 | −198.724985 |
| 2.2 | −198.899754 | −198.485540 | −198.675193 | −198.723453 |
| 2.4 | −198.896158 | −198.449168 | −198.672091 | −198.721616 |
| 2.6 | −198.894498 | −198.419710 | −198.670745 | −198.720790 |
| 2.8 | −198.893750 | −198.396337 | −198.669977 | −198.720414 |
| 3.0 | −198.893422 | −198.378155 | −198.669397 | −198.720235 |
| 3.2 | −198.893266 | −198.364269 | −198.668934 | −198.720163 |
| 3.4 | −198.893185 | −198.353794 | −198.668572 | −198.720153 |
| 3.6 | −198.893150 | −198.345902 | −198.668283 | −198.720171 |
| 3.8 | −198.893136 | −198.339875 | −198.668039 | −198.720197 |
| 4.0 | −198.893132 | −198.335138 | −198.667823 | −198.720222 |

[a] 1s orbitals frozen.

[1] P.-F. Loos, M. Comin, X. Blase, and D. Jacquemin, J. Chem. Theory Comput. **17**, 3671 (2021).
